# Supplementary material for: KROMA: Ontology Matching with Knowledge Retrieval and Large Language Models
Source: arXiv:2507.14032 source file (2025-09-11)
Supplement: Supplementary file 1 [file appendix.tex]

\begin{table}[!ht]
  \centering
  \caption{All systems (codes) across 6 datasets.}
  % \scriptsize
  \setlength{\tabcolsep}{2pt}
  \begin{tabular}{l l c c c}
    \toprule
    \textbf{Dataset} & \textbf{Model} & \textbf{$P$} & \textbf{$R$} & \textbf{$F_1$} \\
    \midrule
    \multirow{8}{*}{Mouse-Human}
      & KL3.3   & 90.78 & 99.50 & \textbf{94.94} \\
      & KNR3.3  & 92.34 & 90.16 & 91.25 \\
      & KNB3.3  &100.00 & 76.36 & 86.59 \\
      & KL3.1   & 90.42 & 99.00 & 94.50 \\
      & KL2.0   &100.00 & 87.34 & 93.24 \\
      & ML3.1   &100.00 & 87.50 & 92.20 \\
      & OL2.0   & 91.40 & 89.10 & 90.20 \\
      & L4G3.5  & 90.82 & 87.46 & 89.11 \\
    \midrule
    \multirow{8}{*}{NCIT-DOID}
      & KL3.3   & 97.59 & 99.69 & \textbf{98.63} \\
      & KNR3.3  & 93.20 & 96.90 & 95.01 \\
      & KNB3.3  & 83.33 &100.00 & 90.91 \\
      & KL3.1   & 97.43 & 99.08 & 98.24 \\
      & KG2     & 84.76 & 86.32 & 85.53 \\
      & ML3.1   & 96.40 & 93.20 & 94.80 \\
      & LLFT    & 86.10 & 62.00 & 72.10 \\
      & L4G3.5  & 86.19 & 80.06 & 83.01 \\
    \midrule
    \multirow{6}{*}{Nell-DBpedia}
      & KL3.3   & 94.32 &100.00 & \textbf{97.08} \\
      & KNR3.3  & 97.46 & 91.27 & 94.26 \\
      & KNB3.3  & 91.17 & 96.12 & 93.58 \\
      & KL2.0   & 95.50 & 96.55 & 96.02 \\
      & OL2.0   &100.00 & 92.20 & 96.00 \\
      & L4G3.5  &100.00 & 89.14 & 94.26 \\
    \midrule
    \multirow{5}{*}{YAGO-Wikidata}
      & KL3.3   & 91.80 & 99.60 & 95.54 \\
      & KNR3.3  & 93.50 & 90.50 & 91.98 \\
      & KNB3.3  & 90.50 & 89.00 & 89.74 \\
      & KL3.2   & 89.09 & 98.00 & 93.33 \\
      & L4L2    &100.00 & 85.52 & 92.19 \\
    \midrule
    \multirow{9}{*}{ENVO-SWEET}
      & K4mini  & 87.23 &100.00 & \textbf{93.18} \\
      & KNR4mini& 86.90 & 98.00 & 92.12 \\
      & KNB4mini& 82.00 & 88.00 & 84.89 \\
      & KL3.1   & 87.11 & 96.19 & 91.43 \\
      & KL2.0   & 92.50 & 78.72 & 85.06 \\
      & KM7     & 87.19 & 99.59 & 92.98 \\
      & ML3.1   & 80.30 & 59.50 & 83.70 \\
      & OL2.0   & 43.10 & 61.30 & 51.10 \\
      & L4M7    & 59.00 & 51.67 & 55.09 \\
    \midrule
    \multirow{5}{*}{MI-MatOnto}
      & KL3.3   & 45.74 & 92.69 & \textbf{61.25} \\
      & KNR3.3  & 44.80 & 91.40 & 59.95 \\
      & KNB3.3  & 42.00 & 85.00 & 55.00 \\
      & KL3.2   & 56.36 & 62.00 & 59.05 \\
      & L4MPT   & 89.70 & 20.19 & 32.97 \\
    \bottomrule
  \end{tabular}
  \label{tab:all_models}
\end{table}
